# Supplementary material for: Predicting the phase behavior of mixtures of active spherical particles
Source: arXiv:1609.03867 ancillary file (2020-04-02)
Supplement: Supplementary file 1 [file SI.pdf]

# Mechanical and chemical equilibrium in mixtures of active spherical particles: predicting phase behaviour from bulk properties alone

## Supplemental Material

Berend van der Meer,<sup>1</sup> Vasileios Prymidis,<sup>1</sup> Marjolein Dijkstra,<sup>1</sup> and Laura Filion<sup>1</sup>

<sup>1</sup>*Soft Condensed Matter, Debye Institute for Nanomaterials Science,  
Utrecht University, Princetonplein 5, 3584 CC Utrecht, The Netherlands*

### I. THE NORMAL COMPONENT OF THE LOCAL PRESSURE TENSOR

Recent theoretical work has established that mechanical pressure is a state function for systems of self-propelled particles that do not experience torque [1]. Moreover, it was recently demonstrated that when such a system undergoes phase separation, the coexisting phases have the same bulk pressure [2]. Here, we expand on the established literature and present an expression for the local pressure of a binary active system with only isotropic interactions. Our expression reproduces the pressure for systems of a single species [3], and, when spatially averaged over the whole system, also amounts to the known expressions for the pressure of non-confined systems [4, 5].

Consider a binary system in  $d$  dimensions with  $N_1$  particles of species 1 and  $N_2$  particles of species 2, whose equations of motion are given by Eqs. 1 and 2 of the main text. These equations should be now viewed with the appropriate generalization in  $d$  dimensions and with  $U(r)$  being an arbitrary pair-wise potential, with  $r = |\mathbf{r}_i - \mathbf{r}_j|$  the center-of-mass distance between particle  $i$  and  $j$ . The only difference between the two species is the value of the self-propulsion force, such that  $f_i = f^{(1)}$  for  $i \in N_1$  and  $f_j = f^{(2)}$  for  $j \in N_2$ , with  $f^{(1)} \neq f^{(2)}$ . For convenience, we also define the (solid) angle between the axis of self-propulsion  $\hat{\mathbf{u}}(t)$  and a fixed coordinate system as  $\Omega(t)$ .

Let us now define the microscopic density field for the two species, which we denote as  $\Psi^{(1)}(\mathbf{r}, \Omega)$  and  $\Psi^{(2)}(\mathbf{r}, \Omega)$ , such that

$$\Psi^{(1)}(\mathbf{r}, \Omega) = \left\langle \sum_{i=1}^{N_1} \delta(\mathbf{r} - \mathbf{r}_i) \delta(\Omega - \Omega_i) \right\rangle \quad (\text{S1})$$

$$\Psi^{(2)}(\mathbf{r}, \Omega) = \left\langle \sum_{i=1}^{N_2} \delta(\mathbf{r} - \mathbf{r}_i) \delta(\Omega - \Omega_i) \right\rangle, \quad (\text{S2})$$

where the average is over different noise realizations. Following standard procedures [6, 7], we find that the time evolution of these fields follows from the equations

$$\partial_t \Psi^{(\alpha)}(\mathbf{r}, \Omega) = -\nabla \cdot \left[ \beta D_0 \left( -\nabla U(\mathbf{r}) + f^{(\alpha)} \hat{\mathbf{u}}(\Omega) \right) \Psi^{(\alpha)}(\mathbf{r}, \Omega) - D_0 \nabla \Psi^{(\alpha)}(\mathbf{r}, \Omega) \right] + D_r \partial_\Omega^2 \Psi^{(\alpha)}(\mathbf{r}, \Omega) \quad (\text{S3})$$

where  $\alpha = 1, 2$ . For later convenience, we now define the moments

$$\rho^{(\alpha)}(\mathbf{r}) = \int d\Omega \Psi^{(\alpha)}(\mathbf{r}, \Omega), \quad (\text{S4})$$

$$\mathbf{m}^{(\alpha)}(\mathbf{r}) = \int d\Omega \hat{\mathbf{u}}(\Omega) \Psi^{(\alpha)}(\mathbf{r}, \Omega), \quad (\text{S5})$$

$$\mathbf{s}_{ij}^{(\alpha)}(\mathbf{r}) = \int d\Omega \hat{\mathbf{u}}_i(\Omega) \hat{\mathbf{u}}_j(\Omega) \Psi^{(\alpha)}(\mathbf{r}, \Omega), \quad (\text{S6})$$

where  $i, j$  denote the spatial components of the corresponding vectors and tensors. The field  $\rho^{(\alpha)}(\mathbf{r})$  is the local density of species  $\alpha$  while the field  $\mathbf{m}^{(\alpha)}(\mathbf{r})$  is the corresponding local polarization.

We assume that the system is confined in the  $\hat{z}$  direction by a wall while it is translationally invariant in the dimensions perpendicular to  $\hat{z}$ , *i.e.* periodic boundary conditions are applied. Then, following standard procedures [1, 3], the pressure felt by the wall can be written as

$$P_{\text{wall}} = P_{\text{id}}(z) + P_{\text{vir}, \hat{z}}(z) + \sum_{\alpha} P_{\text{swim}, \hat{z}}^{(\alpha)}(z), \quad (\text{S7})$$

where  $z$  denotes any point in the bulk of the system,

$$P_{\text{id}}(z) = \rho(z) k_B T = \frac{1}{L^{d-1}} \int d\mathbf{r}^{d-1} \rho(\mathbf{r}) k_B T, \quad (\text{S8})$$

is the ideal component of the pressure, where we have spatially integrated over the dimensions that are perpendicular to the  $\hat{z}$  dimension and divided by the surface  $L^{d-1}$  that we integrated over,

$$P_{\text{vir},\hat{z}}(z) = \frac{1}{L^{d-1}} \int_{z'' < z} d\mathbf{r}'' \int_{z' > z} d\mathbf{r}' \rho(\mathbf{r}'') \rho(\mathbf{r}') \partial_z U(\mathbf{r}' - \mathbf{r}''), \quad (\text{S9})$$

is the standard local virial term, and

$$P_{\text{swim},\hat{z}}^{(\alpha)}(z) = \frac{D_0 f^{(\alpha)}}{(d-1)D_r} \left[ -\beta \partial_z U(z) \mathbf{m}_z^{(\alpha)}(z) + \beta f^{(\alpha)} \mathbf{s}_{zz}^{(\alpha)}(z) - \partial_z \mathbf{m}_z^{(\alpha)}(z) \right] \quad (\text{S10})$$

is the local swim pressure of species  $\alpha$ . In Eq. S10  $U(z)$ ,  $\mathbf{m}_z^{(\alpha)}(z)$  and  $\mathbf{s}_{zz}^{(\alpha)}(z)$  have been averaged similarly to Eq. S8.

Now, since the right-hand-side of Eq. S7 is a local quantity, we straightforwardly define the normal component of the local pressure of the system as

$$P_N(z) = P_{\text{id}}(z) + P_{\text{vir},\hat{z}}(z) + \sum_{\alpha} P_{\text{swim},\hat{z}}^{(\alpha)}(z). \quad (\text{S11})$$

In our particle simulations, we divide the simulation box into slabs, and measure the normal component of the pressure for each slab. The contributions of the ideal and swim components of the pressure to each slab can be calculated straightforwardly, while for the virial component we use Ref. 8.

## II. LENNARD-JONES SYSTEM

Here we give a more detailed description of our simulations of the Lennard-Jones system. The binary system we used is comprised of passive particles ( $f = 0$ ) and active particles with self-propulsion force  $f = 10k_B T/\sigma$ . The rotational diffusion coefficient  $D_r$  is given by the Stokes-Einstein relation  $D_r = 3D_0/\sigma^2$ . For such mild self-propulsion the system is dominated by attractions. As a result, we obtain an attraction-driven liquid-gas phase separation.

For the direct coexistence simulations between the liquid and the gas phases we simulated approximately 8000 particles in a three-dimensional elongated box with dimensions  $L_{\hat{z}} = 12L_{\hat{y}} = 12L_{\hat{x}}$ . This choice for the dimensions of the box ensures that two flat interfaces form that span the shorter dimension [2]. For the highest density (smallest simulation box) we consider, the dimensions of the box are approximately  $12\sigma \times 12\sigma \times 144\sigma$ . Thus, the short axis of the box is much larger than the persistence length of the active particles, which is  $\beta D_0 f / 2D_r \approx 1.67\sigma$ . The Péclet number of the active particles is  $\text{Pe} = 3\beta D_0 f / \sigma D_r = 10$ . Note that we performed direct coexistence simulations for system compositions  $x = 0 - 0.4$ , and total densities  $\rho\sigma^3 = 0.20, 0.30$  and  $0.40$ . These simulations were initiated from a configuration where all particles are located within a dense slab and ran for approximately  $3500\tau$ , where  $\tau = \sigma^2/D_0$ , using a integration time step of  $10^{-5}\tau$ . We collected data only for the last  $500\tau$ .

For the reservoir simulations we simulated approximately 4000 particles. Here we “tuned” the density of the reservoir by measuring the partial densities within the middle section of the binary phase. If the partial density of one of the species became too high, particles of this species were removed randomly. If the partial density of one of the species became too low, particles of this species were added randomly. After a steady state reservoir density was obtained, we stopped removing and adding particles, and checked that the reservoir densities remained constant.

## III. WEEKS-CHANDLER-ANDERSEN SYSTEM

Here we give a more detailed description of our study of the Weeks-Chandler-Andersen system. The binary system we used comprised of slow particles with self-propulsion force  $f_s = 120k_B T/\sigma$  and fast particles with self-propulsion force  $f_f = 160k_B T/\sigma$ . The rotational diffusion coefficient  $D_r$  is given by the Stokes-Einstein relation  $D_r = 3D_0/\sigma^2$ . The Péclet numbers of the fast and slow active particles are  $\text{Pe}_{f,s} = 3\beta D_0 f_{f,s} / \sigma D_r = 160$  and  $120$ , respectively. We chose such a set of forces for two reasons. First of all, such a choice ensures that even the slow species undergoes motility induced phase separation (MIPS) into a fluid and a crystal phase (see e.g. the state diagram of MIPS in Ref. 9). As a result, we can probe the full spectrum of compositions of the binary mixture. Secondly and more importantly, such high self-propulsions result in relatively fast dynamics of the system, so that our reservoir simulations can access a large number of configurations within reasonable computational time.

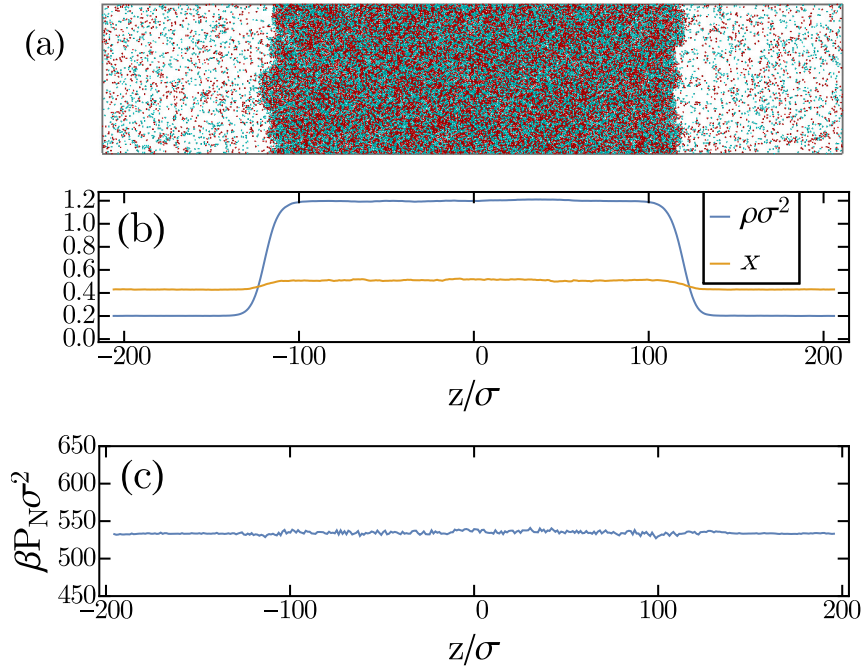

FIG. S1: (a) MIPS of an active-active binary mixture with overall fraction  $x = 0.5$  and overall density  $\rho\sigma^2 = 0.75$ . Red particles are “fast” swimmers with self-propulsion force  $f_f = 160k_B T/\sigma$  and blue particles are “slow” swimmers with self-propulsion force  $f_s = 120k_B T/\sigma$ . The system contains approximately 30000 particles. (b) The corresponding density ( $\rho$ ) and composition profile ( $x$ ) along the long direction  $z$ . (c) The corresponding normal pressure profile along the long direction  $z$ .

### A. Direct coexistence simulations

For the direct coexistence simulations between the fluid and the crystal phases, we simulated approximately 30000 particles in a two dimensional elongated box with dimensions  $L_z = 5L_y$ . This choice for the dimensions of the box was done such that two flat interfaces are created that span the shorter dimension space [2]. Note that we also observe the formation of gas bubbles in the crystal phase, which have been reported in Ref. 2.

In order to construct the phase diagram we performed direct coexistence simulations for system compositions  $x = 0 - 1$  with an interval of 0.1, and total densities  $\rho\sigma^2 = 0.45, 0.6$  and  $0.75$ . For the highest density we consider, the dimensions of the box are approximately  $90\sigma \times 450\sigma$ . Thus, the short axis of the box is larger than the persistence lengths of the active particles, which are  $\beta D_0 f_f / D_r \approx 53.3\sigma$  and  $\beta D_0 f_s / D_r = 40\sigma$ , for the fast and slow species respectively. The simulations were initiated from a configuration where all particles are part of a hexagonal crystal and ran for approximately  $1500\tau$ . We collected data only for the last  $500\tau$ , where  $\tau = \sigma^2 / D_0$ , using a integration time step of  $10^{-5}\tau$ . The long running times are necessary for the relaxation of the compositions of the coexisting phases.

We then measured the local densities of the two species and the normal component of the pressure by dividing the box into slabs of length  $\sigma$  across the long  $z$ -axis and measuring the corresponding quantities for each slab. Typical results for such measurements as well as a snapshot of the system in direct coexistence are shown in Fig. S1. From the results of these direct coexistence simulations we construct the phase diagram, as shown in Fig. 5(a) of the main text.

### B. Reservoir simulations and predicting the phase diagram

In this section we describe how we constructed the two surfaces shown in Fig. 5(b) and the full black lines of Fig. 5(a) of the main text. For a reservoir simulation we place a binary phase in coexistence with a reservoir of only one species of particles. Similarly to the case of the Lennard-Jones particles, the two parts of the system were separated by a semipermeable wall, that repels the species that is absent in the reservoir. In addition to the repulsion, we also apply a torque to the particles of this species, that reorients these particles away from the wall. This torque was applied in order to minimize the accumulation of particles on the wall. Reassuringly, we find that the applied torque has no effects on the bulk part of the binary phase, as the orientation of the particles relaxes rapidly as we move away

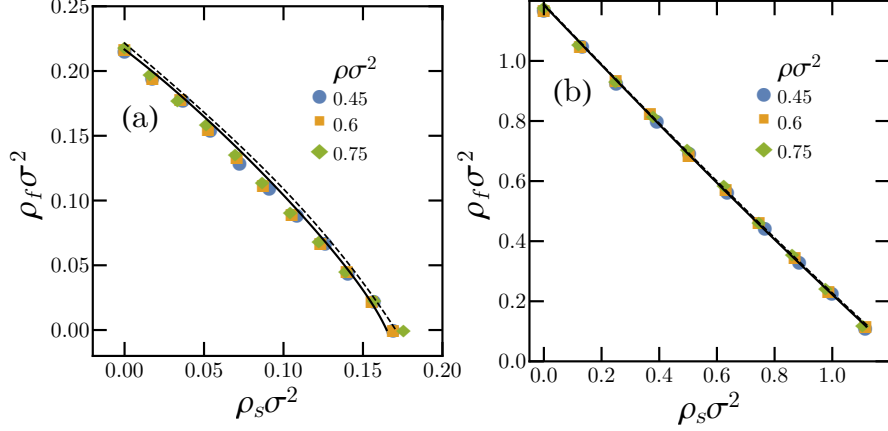

FIG. S2: MIPS: Predicted binodal lines before (dashed lines) and after (full lines) applying a correction to the pressure of the reservoir simulations. Markers denote the results from direct coexistence simulations. (a) covers the low-density region of the phase diagram and (b) the high-density region.

from the wall.

To construct the surface that corresponds to the gas, we ran simulations of a gas phase in contact with a reservoir in order to acquire the reservoir densities for fast and slow swimmers. The gas phases we considered had compositions in the regime  $x \in (0.1 - 0.9)$  and densities  $\rho \sigma^2 = 0.05 - 0.5$  (see shaded area in Fig. 5(a) of the main text). The interval between the points we considered was 0.1 for the composition and 0.02 – 0.05 for the density. We find that for total density  $\rho \sigma^2 > 0.4$  the system spontaneously phase separates so we cannot probe this high-density regime. For each gas phase, which corresponds to a point in the  $(x, \rho \sigma^2)$  grid, we ran two simulations, one in contact with a reservoir of fast swimmers and one in contact with a reservoir of slow swimmers. Each simulation provided us with a value for the density of the corresponding reservoir and also a value for the normal pressure in the bulk. The values for the pressures were reassuringly in close agreement, since we simulated the same binary bulk phase in both simulations. Thus a pair of such simulations provided us with a hypersurface  $(\rho_f^{\text{res}}, \rho_s^{\text{res}}, \beta P \sigma^2)$ , which is a function of the variables  $x$  and  $\rho \sigma^2$ . As the value of the pressure  $\beta P \sigma^2$  we take the average from the two simulations. This surface can be well fitted by a second degree polynomial. The red surface shown in Fig. 5(b) of the main text is the fitted polynomial.

For the crystal phase we perform a similar approach. We simulate the binary bulk crystal in contact with a reservoirs of slow and fast particles separately. The points we simulated were in the interval of compositions  $x \in (0.1 - 0.9)$  and densities  $\rho \sigma^2 = 1 - 1.30$ , with intervals 0.1 for the composition and 0.02 for the density (see shaded area in Fig. 5(a) of the main text). Again, the results of the simulations give us a hypersurface which we again fit with a second degree polynomial. This polynomial is the blue surface shown in Fig. 5(b) of the main text.

The intersection of the two surfaces is the line where the reservoir densities of both species and pressures of the binary crystal and gas phases are equal. Thus, it should correspond to the binodals of the phase diagram. The lines on every  $(\rho_f^{\text{res}}, \rho_s^{\text{res}}, \beta P \sigma^2)$  surface can be converted back into lines on the  $x, \rho \sigma^2$  and subsequently the  $\rho_f \sigma^2, \rho_s \sigma^2$  representation of the phase diagram. The resulting phase boundaries are drawn in Fig. 5(a) of the main text in order to compare them with the results from the direct coexistence simulations. A more detailed view can be seen in Fig. S2.

We find that the predicted high-density binodal (dashed black line in Fig. S2(b)) is in excellent agreement with the points from the direct coexistence simulations. The low-density binodal (dashed black line in Fig S2(a)) slightly deviates to higher densities. We attribute this discrepancy to finite-size effects in our simulations. We find that on average, the reservoir simulations measure a higher pressure of the binary crystal than the direct coexistence simulation despite having equal densities and compositions. This difference is caused by the different tangential dimensions of the box between the reservoir and the direct coexistence simulation. A typical direct coexistence simulation has a box length in the tangential dimension three times larger than the reservoir simulation. Note that the pressure difference is minute: on average we measure a pressure difference  $\Delta P \beta \sigma^2 \sim 4$ , while the pressure of the system in coexistence is in the range  $P \beta \sigma^2 \sim 400 - 700$ . In order estimate the magnitude of this finite size effect on the binodals, we make a crude correction by shifting vertically the crystal (blue) surface of Fig. 5(b) of the main text by a constant which is equal to the average pressure difference. This correction subsequently alters the intersection of the two surfaces, and shifts the initially predicted binodals to the full lines shown in Fig. S2. This indeed appears to correct for the majority

of the discrepancy between the predicted and measured coexistence lines. It should be noted that this correction is not included in the coexistence lines reported in Fig. 5(b) of the main text.

- 
- [1] A. P. Solon, Y. Fily, A. Baskaran, M. E. Cates, Y. Kafri, M. Kardar, and J. Tailleur, *Nat. Phys.* **11**, 673 (2015).
  - [2] J. Bialké, J. T. Siebert, H. Löwen, and T. Speck, *Phys. Rev. Lett.* **115**, 098301 (2015).
  - [3] A. P. Solon, J. Stenhammar, R. Wittkowski, M. Kardar, Y. Kafri, M. E. Cates, and J. Tailleur, *Phys. Rev. Lett.* **114**, 198301 (2015).
  - [4] R. G. Winkler, A. Wysocki, and G. Gompper, *Soft Matter* **11**, 6680 (2015).
  - [5] G. Falasco, F. Baldovin, K. Kroy, and M. Baiesi, *arXiv:1512.01687*.
  - [6] D. S. Dean, *J. Phys. A: Math. Gen.* **29**, L613 (1996).
  - [7] A. M. Menzel, *Phys. Rev. E* **85**, 021912 (2012).
  - [8] T. Ikeshoji, B. Hafskjold, and H. Furuho, *Molecular Simulation* **29**, 101 (2003).
  - [9] G. S. Redner, M. F. Hagan, and A. Baskaran, *Phys. Rev. Lett.* **110**, 055701 (2013).
